# Supplementary material for: The Brain Tumor Sequence Registration (BraTS-Reg) Challenge: Establishing Correspondence Between Pre-Operative and Follow-up MRI Scans of Diffuse Glioma Patients
Source: arXiv:2112.06979 source file (2024-04-17)
Supplement: Supplementary file 1 [file appendix_B.tex]

\section*{Appendix B.}

\emph{To Do: Contributions of all authors.}
